# Supplementary material for: Leveraging Video Descriptions to Learn Video Question Answering
Source: arXiv:1611.04021 source file (2016-12-19)
Supplement: Supplementary file 1 [file supp.pdf]

# Technical Report: Leveraging Video Descriptions to Learn Video Question Answering

**Kuo-Hao Zeng**[*†], **Tseng-Hung Chen**[*], **Ching-Yao Chuang**[*]

**Yuan-Hong Liao**[*], **Juan Carlos Niebles**[†], **Min Sun**[*]

[*]Department of Electrical Engineering, National Tsing Hua University
[†]Department of Computer Science, Stanford University
{khzeng, jniebles}@cs.stanford.edu
{s104061544@m104, s102061145@m102, s102061137@m102, sunmin@ee}.nthu.edu.tw

## Auto-generated Questions vs. Human-generated Questions

We compare auto-generated questions (Auto-QG) with human-generated questions (Human-QG) by distribution and question length.

### Distribution

Both distributions of Auto-QG and Human-QG are plotted in Fig. 1. The distributions are similar with a few noticeable differences. For examples, the most frequent question type is *What* and the second one is *Yes/No* type questions, including *Does*, *Do*, *Did*, *Are*, *Were*, *Is* and *Was* for both types of QG. However, Auto-QG has about 13% more questions starting with *Who*. Although Auto-QG does not have exactly the same distribution as Human-QG, it is still a very cost effective way to obtain QA pairs from descriptions.

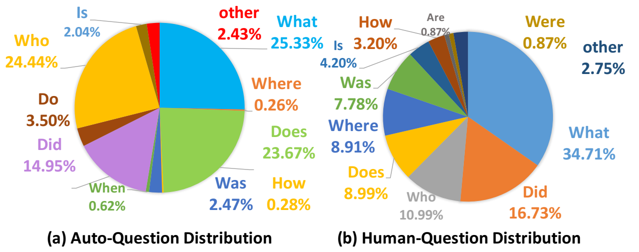


Figure 1: The distributions of auto-generated questions (Left-panel) and human-generated questions (Right-panel).

### Length

The statistic analysis of questions length are listed in Table. 1. It reveals that questions generated by Human-QG are shorter than those generated by Auto-QG. The reason is that human typically generates questions after understanding (but not systematically parsing) descriptions of the video. Hence, the questions tend to be more compact.

Finally, we show more typically examples of Auto-QG (Left-panel) and Human-QG (Right-panel) in Fig. 2.

Copyright © 2017, Association for the Advancement of Artificial Intelligence (www.aaai.org). All rights reserved.

| Length | Max. | Min. | Mean | Std. | Median |
|---|---|---|---|---|---|
| Auto-QG | 36 | 2 | 10.8 | 5.3 | 9 |
| Human-QG | 37 | 2 | 7.3 | 3.2 | 7 |

Table 1: Length analysis of questions for Auto-QG and Human-QG. Max., Min., Mean, Std. and Median denote the maximum, the minimum, the average, the standard deviation and the median length of questions, respectively.

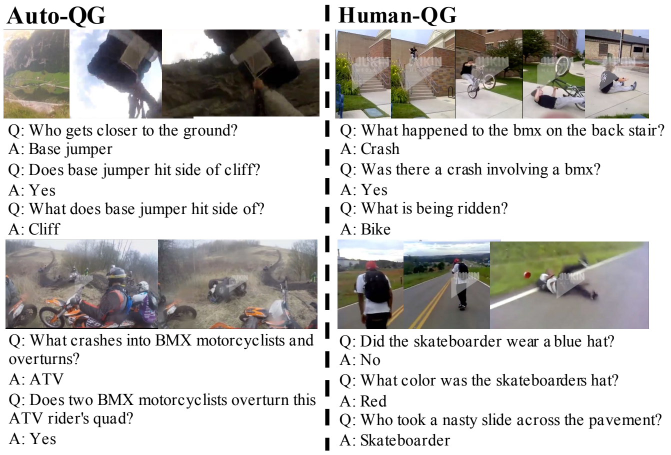


Figure 2: Typical examples for Auto-QG and Human-QG.

## Video-QA examples

We show more typical examples in Fig. 3.

**Description:** This snowboarder skims the surface of a pond until unintentionally cartwheeling and face planting into the water.

**Question:** Who skims the surface of the pond? $\mathbf{Ans_{gt}}$: Snowboarder $\mathbf{Ans_{pred}}$: Snowboarder

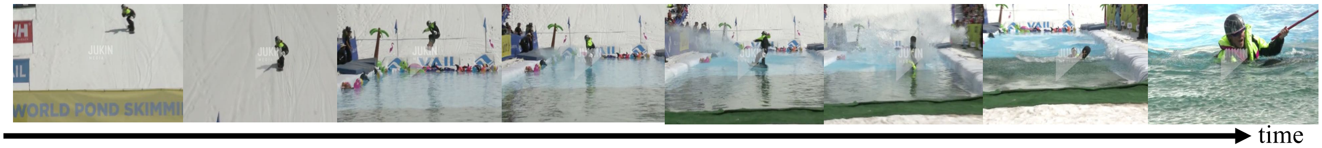


**Description:** These two very brave souls took an incredible jump off a very high bridge overlooking a gorgeous beach.

**Question:** What did the two guys jump off of? $\mathbf{Ans_{gt}}$: Bridge $\mathbf{Ans_{pred}}$: Bridge

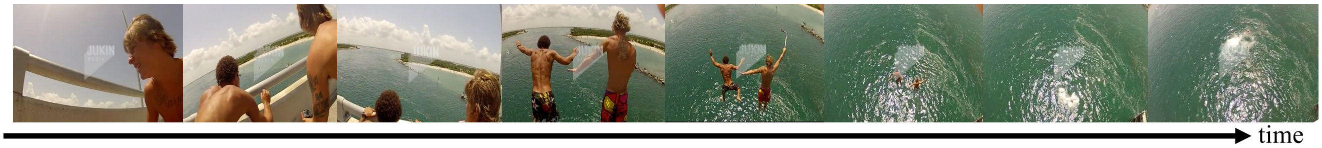


**Description:** Maddie the Labrador Retriever knows that if you want something done right, you have to do it yourself. So when she wanted to take a dip on a hot summer day, she took it upon herself to grab the hose and fill up the kiddie pool in the backyard.

**Question:** What does the yellow labrador fill up the kiddie pool with? $\mathbf{Ans_{gt}}$: Water $\mathbf{Ans_{pred}}$: Water

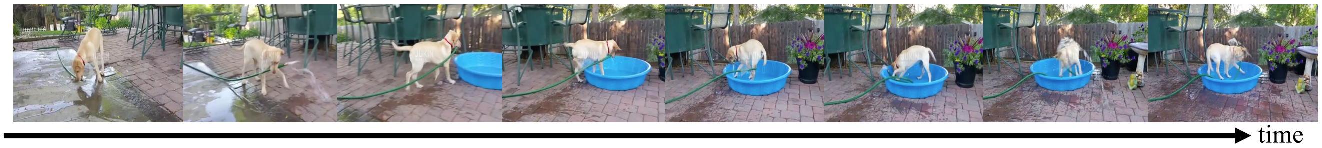


**Description:** A boy at a skatepark rides his scooter up a ramp to attempt a backflip, but bails halfway up and falls butt-first to the ground.

**Question:** Did the kid fall on his butt? $\mathbf{Ans_{gt}}$: Yes $\mathbf{Ans_{pred}}$: Yes

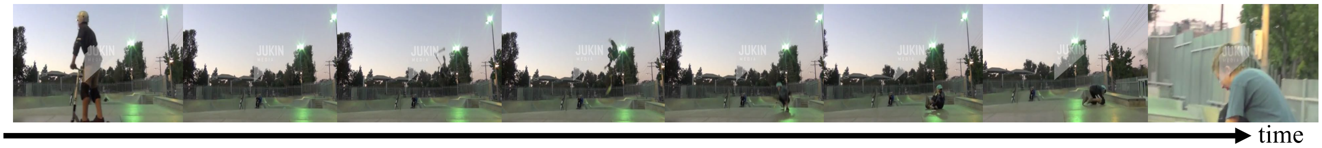


**Description:** This basketball player was successful in dunking a ball into the hoop, but he wasn't as graceful on his landing as he faceplanted hard on the gym floor.

**Question:** Was the basketball player successful in dunking a ball into the hoop? $\mathbf{Ans_{gt}}$: Yes $\mathbf{Ans_{pred}}$: Yes

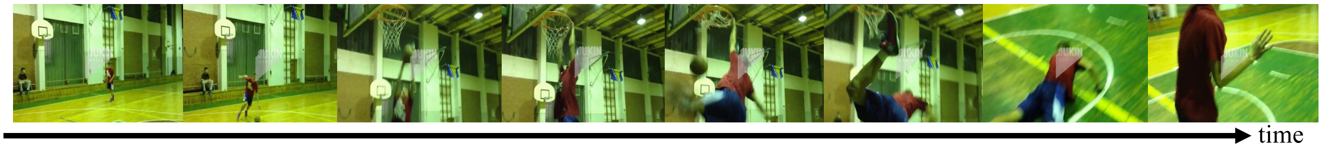


**Description:** This athlete runs and leaps off a concrete ledge on a roof, but ends up mistiming the stunt and crashes shoulder first into another wall nearby.

**Question:** Will athlete do parkour again? $\mathbf{Ans_{gt}}$: No $\mathbf{Ans_{pred}}$: No

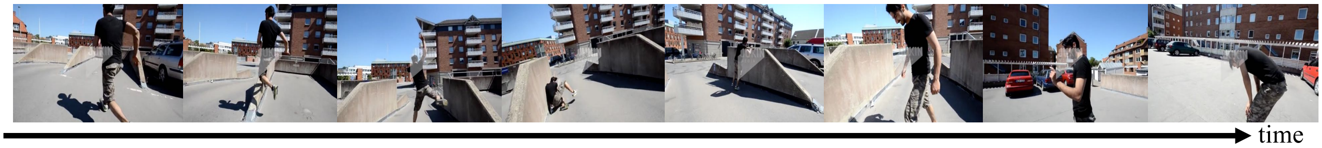


Figure 3: More qualitative Video QA results. In each row, we show a typical example with corresponding description, question, predicted answer and ground truth answer. In total, we show 3 *Others* type examples and 3 *Yes/No* type examples.
